# Supplementary material for: Vox-E: Text-guided Voxel Editing of 3D Objects
Source: arXiv:2303.12048 source file (2023-09-19)
Supplement: Supplementary file 1 [file supp_attn_duck.tex]

\begin{figure*} %
\centering
\rotatebox{90}{\whitetxt{xxx}2D Edit}
\jsubfig{\includegraphics[height=2.78cm]{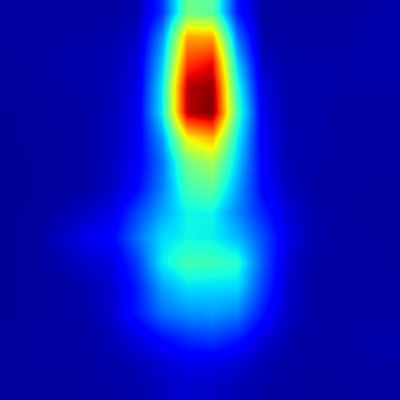}}{}\hfill
\jsubfig{\includegraphics[height=2.78cm]{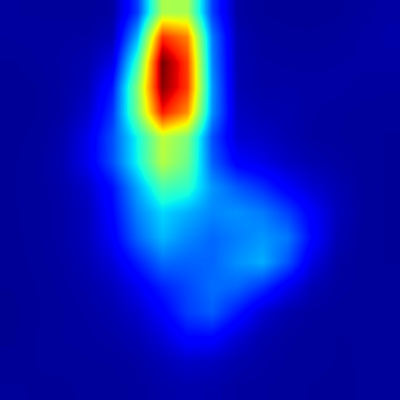}}{} \hfill
\jsubfig{\includegraphics[height=2.78cm]{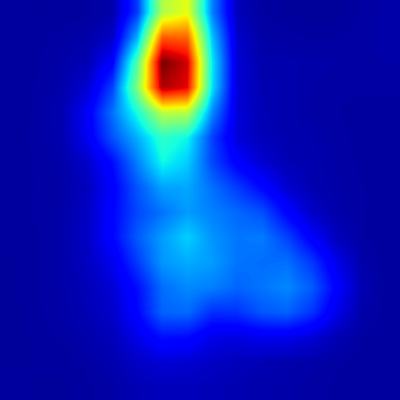}}{} \hfil
\jsubfig{\includegraphics[height=2.78cm]{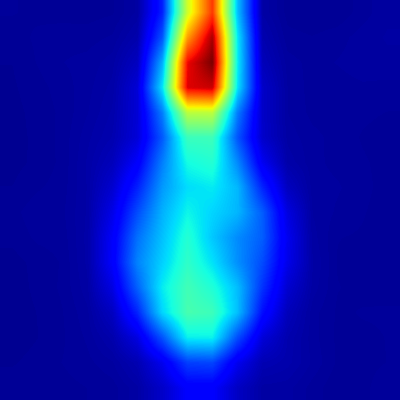}}{}\hfill
\jsubfig{\includegraphics[height=2.78cm]{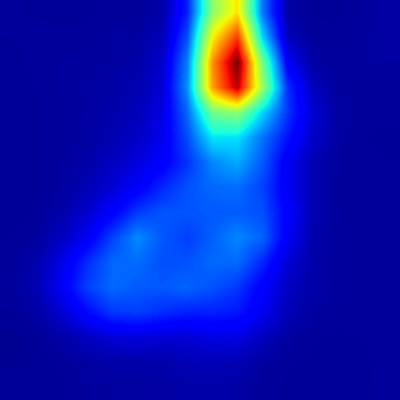}}{}\hfill
\jsubfig{\includegraphics[height=2.78cm]{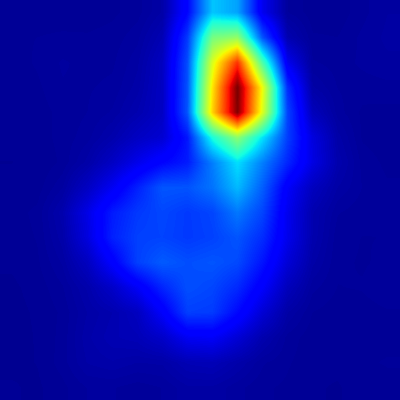}}{}
\rotatebox{90}{\whitetxt{xxx}3D Edit}
\jsubfig{\includegraphics[height=2.78cm]{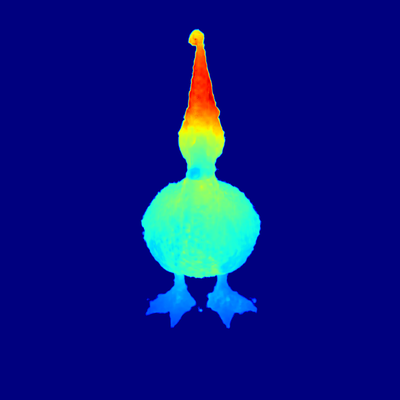}}{} \hfill
\jsubfig{\includegraphics[height=2.78cm]{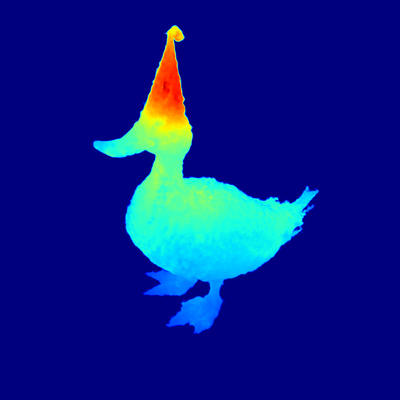}}{}\hfill
\jsubfig{\includegraphics[height=2.78cm]{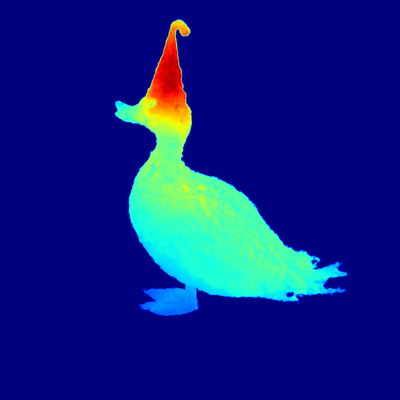}}{} \hfill
\jsubfig{\includegraphics[height=2.78cm]{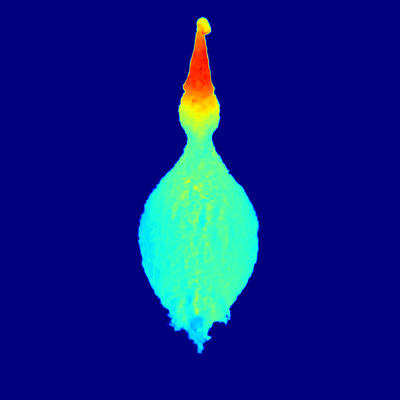}}{}\hfill
\jsubfig{\includegraphics[height=2.78cm]{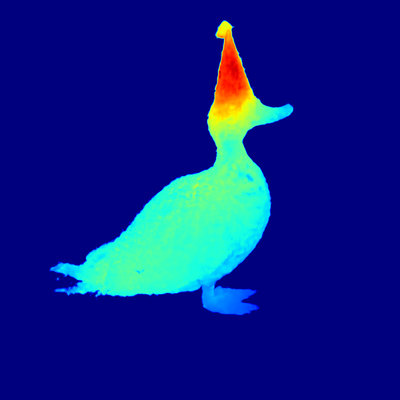}}{}\hfill
\jsubfig{\includegraphics[height=2.78cm]{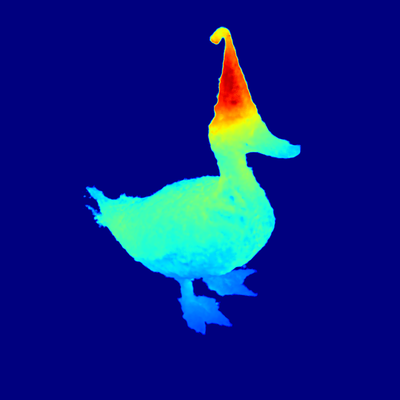}}{}
\rotatebox{90}{\whitetxt{xxx}2D Object}
\jsubfig{\includegraphics[height=2.78cm]{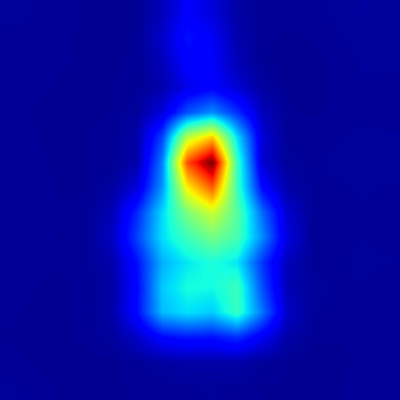}}{}\hfill
\jsubfig{\includegraphics[height=2.78cm]{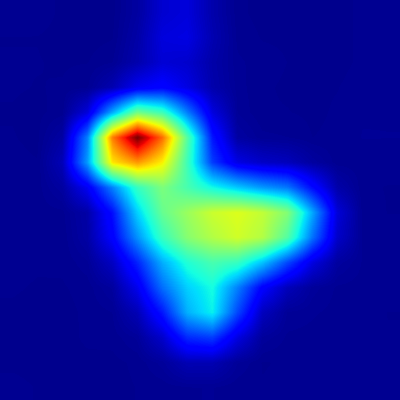}}{} \hfill
\jsubfig{\includegraphics[height=2.78cm]{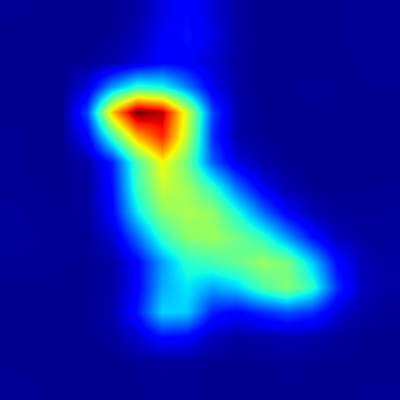}}{} \hfil
\jsubfig{\includegraphics[height=2.78cm]{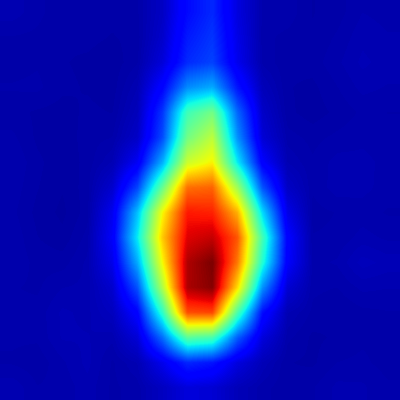}}{}\hfill
\jsubfig{\includegraphics[height=2.78cm]{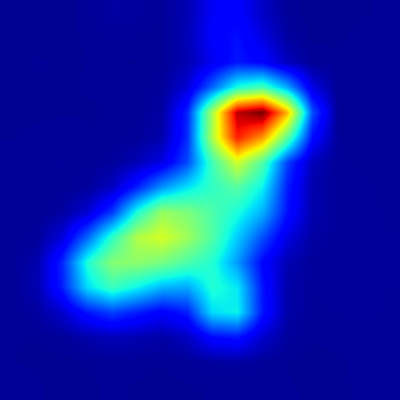}}{}\hfill
\jsubfig{\includegraphics[height=2.78cm]{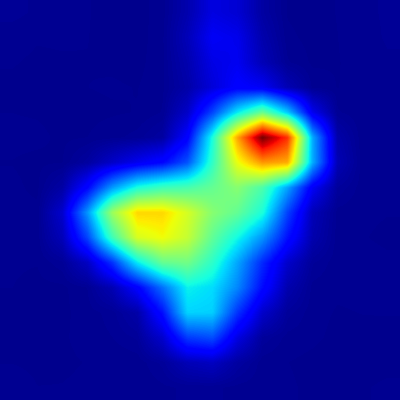}}{}
\rotatebox{90}{\whitetxt{xxx}3D Object}
\jsubfig{\includegraphics[height=2.78cm]{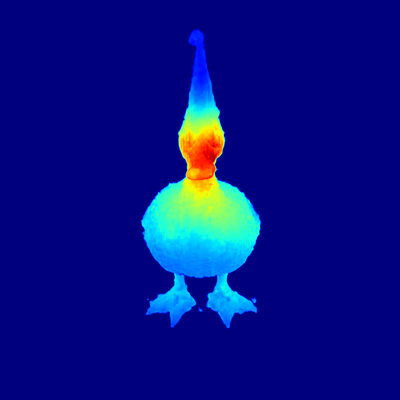}}{} \hfill
\jsubfig{\includegraphics[height=2.78cm]{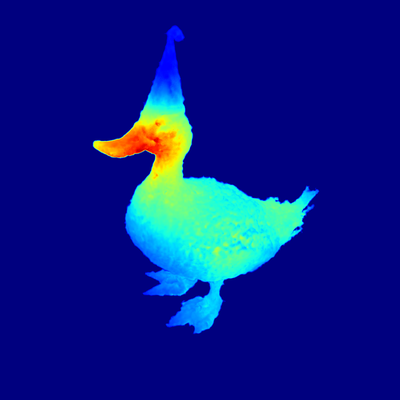}}{}\hfill
\jsubfig{\includegraphics[height=2.78cm]{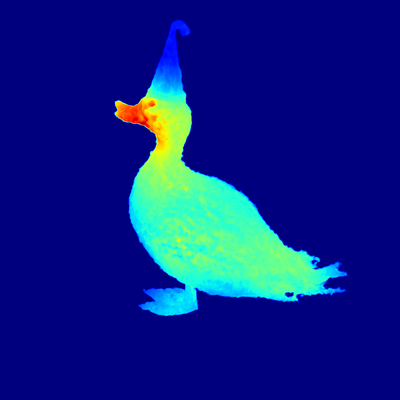}}{} \hfill
\jsubfig{\includegraphics[height=2.78cm]{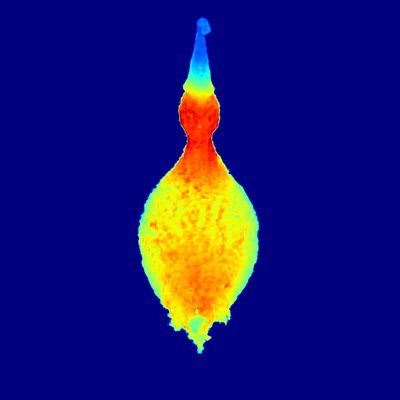}}{}\hfill
\jsubfig{\includegraphics[height=2.78cm]{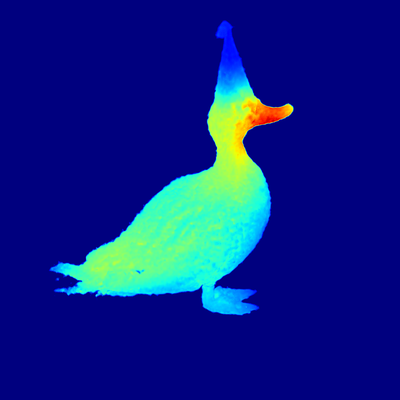}}{}\hfill
\jsubfig{\includegraphics[height=2.78cm]{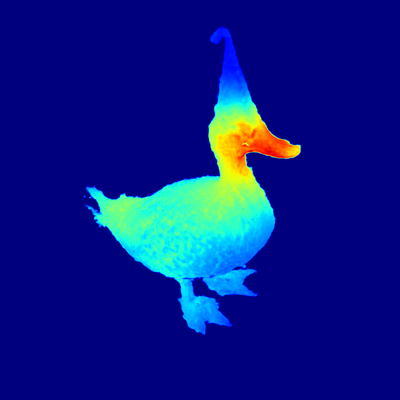}}{}
\rotatebox{90}{\whitetxt{xxx}Blend Edit}
\jsubfig{\includegraphics[height=2.78cm]{images/supp_attn/duck/blend_edit/0.png}}{}\hfill
\jsubfig{\includegraphics[height=2.78cm]{images/supp_attn/duck/blend_edit/30.png}}{} \hfill
\jsubfig{\includegraphics[height=2.78cm]{images/supp_attn/duck/blend_edit/60.png}}{} \hfil
\jsubfig{\includegraphics[height=2.78cm]{images/supp_attn/duck/blend_edit/90.png}}{}\hfill
\jsubfig{\includegraphics[height=2.78cm]{images/supp_attn/duck/blend_edit/120.png}}{}\hfill
\jsubfig{\includegraphics[height=2.78cm]{images/supp_attn/duck/blend_edit/150.png}}{}
\rotatebox{90}{\whitetxt{xxx}Blend Object}
\jsubfig{\includegraphics[height=2.78cm]{images/supp_attn/duck/blend_object/0.png}}{} \hfill
\jsubfig{\includegraphics[height=2.78cm]{images/supp_attn/duck/blend_object/30.png}}{}\hfill
\jsubfig{\includegraphics[height=2.78cm]{images/supp_attn/duck/blend_object/60.png}}{} \hfill
\jsubfig{\includegraphics[height=2.78cm]{images/supp_attn/duck/blend_object/90.png}}{}\hfill
\jsubfig{\includegraphics[height=2.78cm]{images/supp_attn/duck/blend_object/120.png}}{}\hfill
\jsubfig{\includegraphics[height=2.78cm]{images/supp_attn/duck/blend_object/150.png}}{}
\rotatebox{90}{\whitetxt{xxx}Output}
\jsubfig{\includegraphics[height=2.78cm]{images/supp_attn/duck/output/0.png}}{} \hfill
\jsubfig{\includegraphics[height=2.78cm]{images/supp_attn/duck/output/30.png}}{}\hfill
\jsubfig{\includegraphics[height=2.78cm]{images/supp_attn/duck/output/60.png}}{} \hfill
\jsubfig{\includegraphics[height=2.78cm]{images/supp_attn/duck/output/90.png}}{}\hfill
\jsubfig{\includegraphics[height=2.78cm]{images/supp_attn/duck/output/120.png}}{}\hfill
\jsubfig{\includegraphics[height=2.78cm]{images/supp_attn/duck/output/150.png}}{}
\vspace{5pt} 
\caption{\textbf{Visualizing 360 degrees of 3d cross-attention grids and the 2D cross-attention maps used for supervision}.  We visualize the trained 3d cross-attention grids and the corresponding 2D cross-attention maps used as training supervision for the edit region "hat" (top two rows) and the object region "duck" (rows 3 and 4). We also add a blended image of the 3d attention grid and the pre-refinement edit grid for both edit (row 5) and object (row 6) regions. The bottom row shows the output edit.
}
\label{fig:supp_attn}
\end{figure*}
